# Supplementary material for: A Strong Bisimulation for a Classical Term Calculus
Source: arXiv:2101.05754 source file (2024-04-17)
Supplement: Supplementary file 1 [file toappendix.tex]

\gettoappendix {t:control:lambda-m:semantics:confluence}
\gettoappendix {t:control:meaningful:can-sn}
\gettoappendix {t:control:meaningful:can-confluence}
\gettoappendix {l:control:equivalence:permute}
\gettoappendix {l:control:bisimulation:ctxt-closure}
\gettoappendix {l:control:bisimulation:meta-eqsigma}
\gettoappendix {t:control:bisimulation}
\gettoappendix {l:eqnew-stack}
\gettoappendix {l:expan-aux-replacement}
\gettoappendix {l:newrel-eqsigma}
\gettoappendix {l:eqsigma-newrel}
